# Supplementary material for: Defect-induced Fermi level pinning and suppression of ambipolar behaviour in graphene
Source: arXiv:1410.4400 source file (2014-10-16)
Supplement: Supplementary file 1 [file Supporting_Information.pdf]

# Supporting Information

## Defect-induced Fermi level pinning and suppression of ambipolar behavior in graphene

Zakaria Moktadir[1,*,] Shuojin[1] Hang and Hiroshi Mizuta[1,2]

[1] Electronics and Computer Science, Faculty of Applied Physical Sciences, Southampton University, United Kingdom

[2]School of Materials Science, JAIST, Nomi, Ishikawa 923-1292, Japan

*Email:zm@ecs.soton.ac.uk

## Measurements on multi-terminal devices

The multi-probe devices were fabricated using the same processes described in the methods section in the main text. A typical device is shown in the inset of figure S1.

The devices were irradiated with accelerated helium ions with an accelerated voltage of 30 kV. The $He^+$ beam current was maintained at 1 pA. Only the white area indicated in the inset of figure S1 is irradiated to avoid damage to contacts and an increase in the source and drain contact resistance**.**

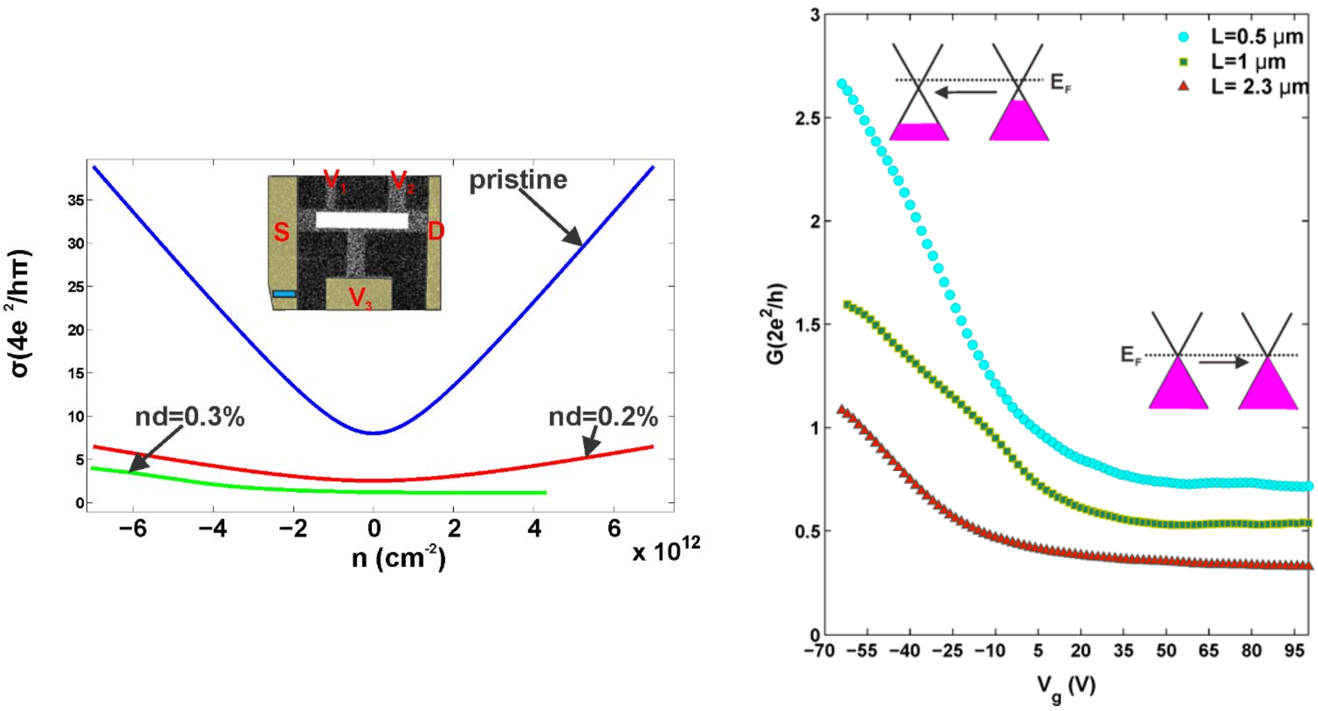


Fig S1: left: conductivity versus carrier density for pristine and defective channels. The inset shows a 5-probe device; the scale bar is 1 um. Right: the conductance versus the gate voltage for nd=0.3 % and for three different channel lengths as indicated. The inset shows a sketch of the Fermi level position with the gate voltage (see main text).

A constant current $I_s$ is injected in the source and the voltage difference ΔV is measured between two probes. The conductivity is given by $\sigma = \frac{L}{w}\frac{I_S}{\Delta V}$, w is the width and L the length of the channel.

In the main panel of figure S1, the conductivity is shown as a function of charge carrier density calculated from $n = C(V_g - V_D)$ where $C \approx 7.2 \times 10^{10}\ cm^{-2}/V$ and $V_D$ is the voltage at the Dirac point[1]. The channel was chosen to be wide (W= 1 um) to exclude the edge effect[2]. The minimum conductivity at the defect concentration of $n_d$= 0.3 % reaches the value of $4e^2/\pi h$. The decrease in the conductivity as a function of defect concentration indicates the absence of zero energy modes in our samples[3].

## Raman spectroscopy of graphene irradiated with helium ions

Raman spectroscopy was performed on freshly exfoliated and irradiated flakes, using a Renishaw instrument with a laser energy of 2.3 eV. Figure S2 shows the Raman spectrum taken for different defect concentrations. The D-peak decreases with increasing defect concentration and the merging of G and D' peaks occurs at large defect concentrations.

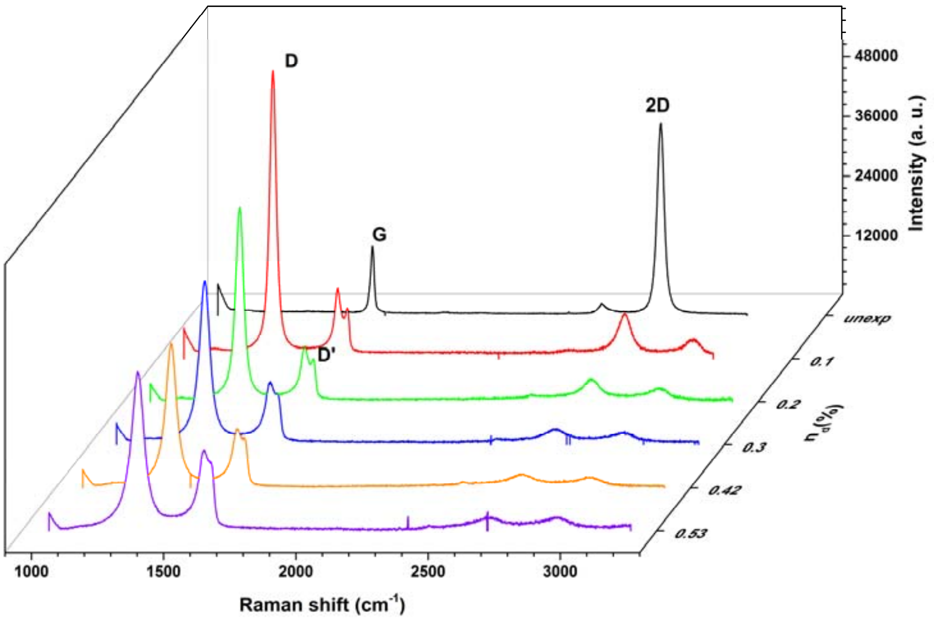


Fig. S2: Raman spectrum versus defect concentration showing the emergence of the D-peak and the D'-peak as the concentration is increased.

**XPS survey of defective graphene samples**:

The X-ray spot size provided by our XPS equipment (Theta probe Thermo Scientific) is larger than the typical size of the exfoliated graphene flakes which are only few microns wide. This induces a loss of accuracy and very low number of counts. We found that a spot size of 100 um is good enough for well resolved spectrum. In addition, this size is below the maximum field of view in the HIM which allows better accuracy during scanning with $He^+$ beam. Therefore we investigated the XPS on a freshly transferred graphene from a copper foil (the graphene is grown by the CVD method) to a Si/$SiO_2$ substrate. To be consistent in our interpretations, we chose areas with minimum ratio I(D)/I(G) using Raman spectroscopy (typically I(D)/I(G) < 1) . The samples are then patterned and coded with metal marks using the same processes used to fabricate graphene nanowire devices. The chosen areas in the same sample are then irradiated inside a HIM using similar doses used in graphene nanowires. The XPS survey is shown in figure S3 for a defect concentration of 0.4%.

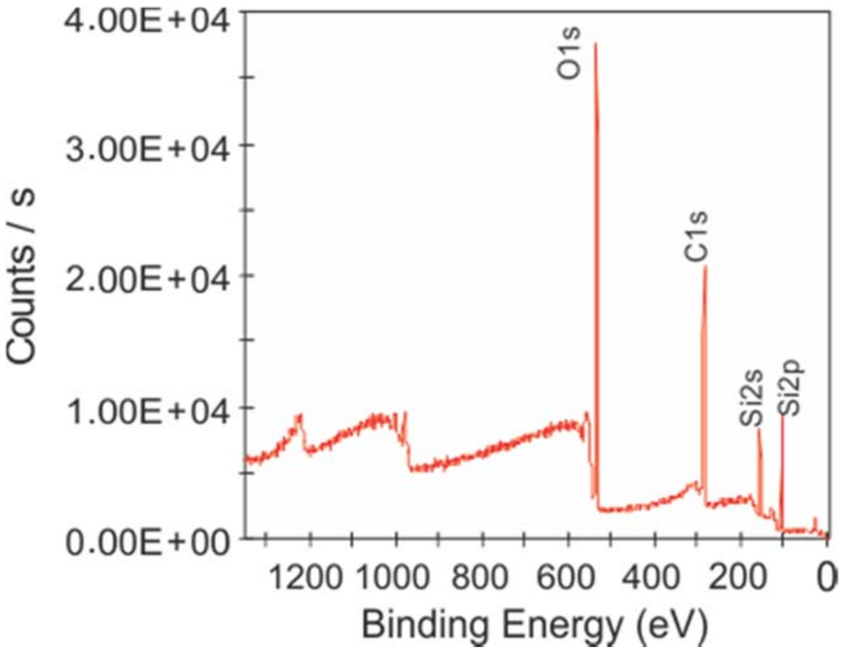


Figure S3: XPS survey of a defective sample with defect concentration of $n_d$=0.4%. The spectrum shows the presence of Carbon, Silicon and Oxygen.

## Determination of $sp^3/sp^2$ ratio using the D-parameter

The D-parameter is the energy difference between the maximum and the minimum values of the first derivative of the C KLL spectrum. A linear relationship exists between this parameter and the ratio of $sp^2/sp^3$ starting from a value of approximately 13 eV for pure $sp^3$ (e.g. diamond) and ending at a value of 21 eV for pure $sp^2$ content[4] (e. g. graphite, Graphene). The C KLL spectrum is shown in figure S4 and its derivative is shown in figure S5 for different defect concentration.

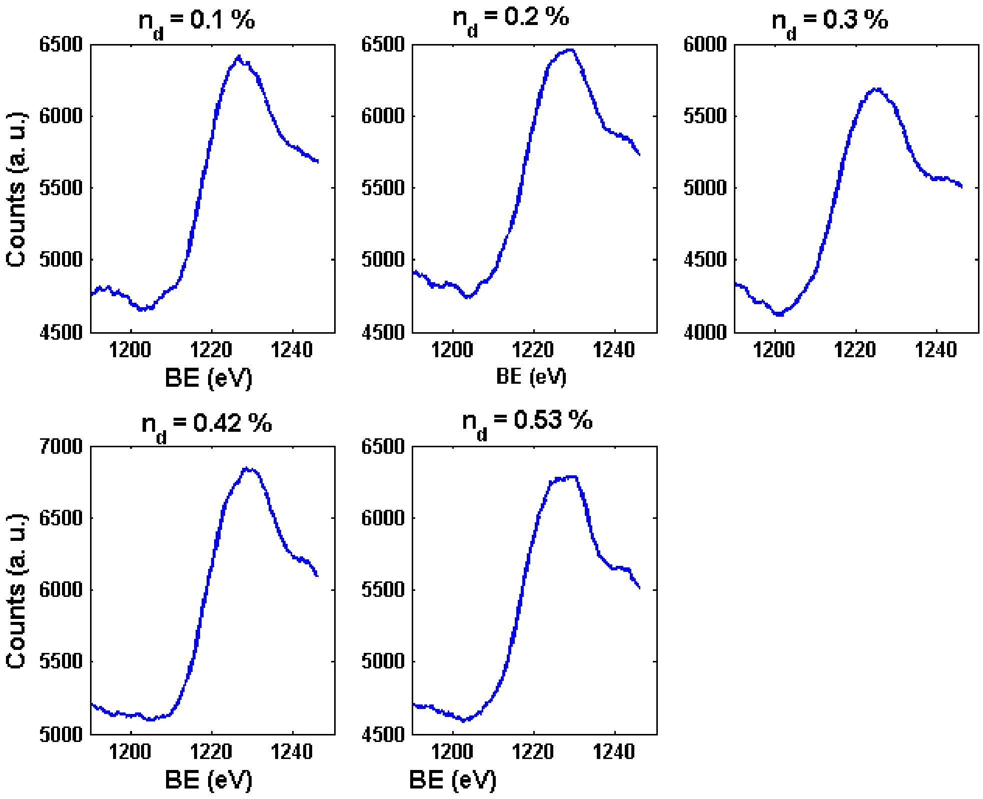


Fig. S4: C KLL Auger spectrum of defective graphene obtained for different values of defect concentrations.

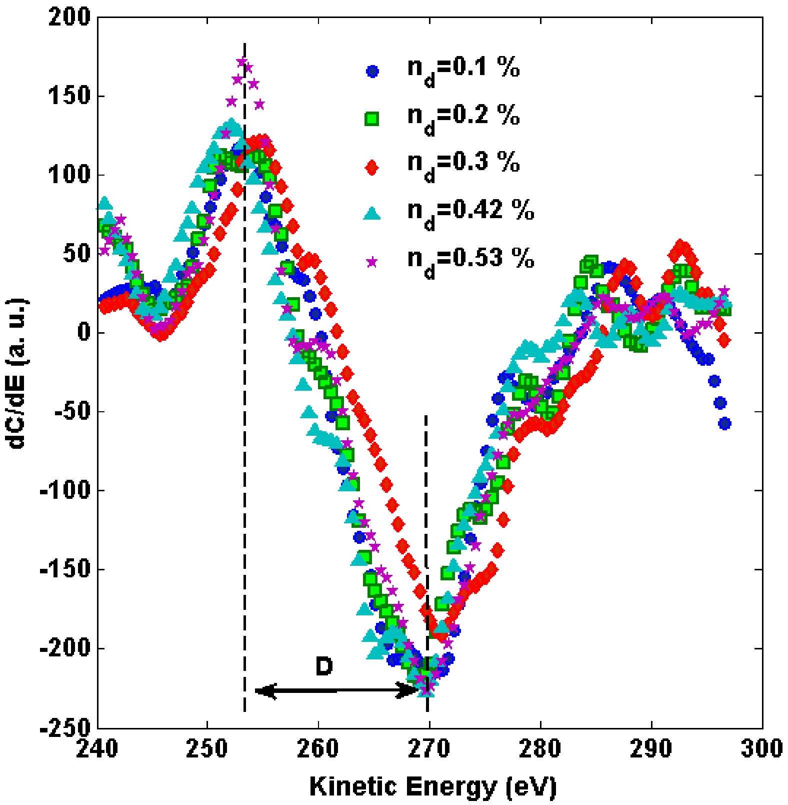


Figure S5: This plot shows the first derivative of the C KLL Auger spectrum versus the kinetic energy of the emitted photoelectrons for different defect concentration. The D-parameter is defined as the energy separation between the minimum of dC/dE and its maximum as indicated.

**References**


1. Sarma, S. Das; Adam, S.; Hwang, E. H. and Enrico, R. Electronic Transport in Two-dimensional Graphene. **2011** Rev. Mod. Phys. 83, 407

2. Guangyu, Xu; Carlos M., Torres Jr.; Jianshi, Tang; Jingwei, Bai; Emil B., Song; Yu, Huang; Xiangfeng, Duan; Yuegang, Zhang; and Kang L., Wang Edge Effect on Resistance Scaling Rules in Graphene Nanostructures Nano Lett. **2011**, 11 (3), 1082.

3. Cresti, A; Ortmann, F.; Louvet, T. ; Tuan, D. V. and Roche, S. Broken Symmetries, Zero-Energy Modes, and Quantum Transport in Disordered Graphene: From Supermetallic to Insulating Regimes Phys. Rev. Lett. **2013**, 110, 196601.

4. A. Mezzi and S. Kaciulis, Surface investigation of carbon films: from diamond to graphite Surf. Interface Anal. **2010**, 42, 1082–10
